# Supplementary material for: Coordination-free Decentralised Federated Learning on Complex Networks: Overcoming Heterogeneity
Source: arXiv:2312.04504 source file (2023-12-07)
Supplement: Supplementary file 1 [file appendix.tex]

%!TEX root = ./tnnls_main.tex
\appendix
